# Supplementary material for: Characterizing Improper Input Validation Vulnerabilities of Mobile Crowdsourcing Services
Source: arXiv:2110.08517 source file (2021-10-19)
Supplement: Supplementary file 1 [file 12_appendix.tex]

\subsection{Privacy Leaks}
\begin{table}[]
\centering
\caption{Flowdroid Source Sink Leak Detection}
\label{tab:flowdroid}
\begin{tabular}{| l | l |}
\hline
 Application         &  Leaks \\ \hline
ancestry & 7 leaks \\ \hline
basket & 0 leaks \\ \hline
neighbors & 0 leaks \\ \hline
fitbit & 5 leaks \\ \hline
gasbuddy & 15 leaks \\ \hline
mapmyrun & 0 leaks \\ \hline
myheritage & 6 leaks \\ \hline
policedetector & 7 leaks \\ \hline
strava & 2 leaks \\ \hline
toifi & 0 leaks \\ \hline
transit & 2 leaks \\ \hline
\end{tabular}
\end{table}
